# Supplementary material for: Hierarchical Overlapping Belief Estimation by Structured Matrix Factorization
Source: arXiv:2002.05797 source file (2022-09-19)
Supplement: Supplementary file 1 [file appendix2.tex]

\newpage

\section{Visualization of Results} 
To compare these methods in more depth, we visualize the final $M$ and colors are based on ground-truth labels. In Figure~\ref{fig:scatter} and Figure~\ref{fig:scatter2}, we project the estimated $M$ into a 3-D space, where each data point represents a message. In each figure, all of the data points seem to lie in a regular tetrahedron (should be regular $K$-polyhedron for more general $K$-belief cases). It is interesting that for NMF, most of the data points cluster around the upper corner. It is obviously difficult  to draw a boundary for the crowded mass. NMTF is a little bit better: data points with different beliefs stretch apart, making their beliefs more separable. We also visualize the learned $\tilde{B}\in\mathbb{R}^{4\times 4}$, and it turns out to be an SVD-like diagonal matrix, which means that pure NMTF only learns the independent  variances aligned with each belief. 

The projection result of BSMF is surprising: data points are evenly located and grouped by colors. They approximately  form a regular tetrahedron. We hypothesize that in the four-dim space, data points should be perfectly aligned with one of the belief bases/parts, and these four bases are conceivably orthogonal in that space. In a word, the results on synthetic data strongly suggest that our model disentangles the latent manifold leading to a better separation of messages by belief sets.

\begin{figure}[t]
	\includegraphics[width=3.4in]{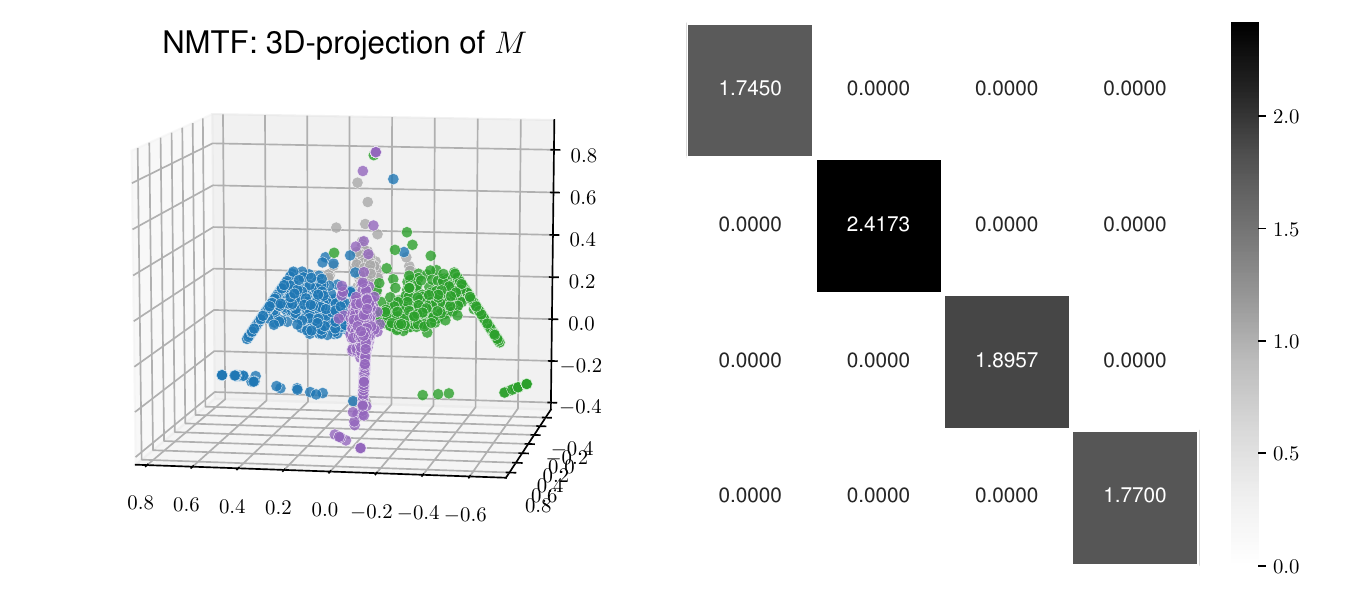}
	\vspace{-0.1in}
	\caption{Visualization of $M$ (Left) and $\tilde{B}$ (Right) for NMTF}
	\label{fig:scatter2}
\end{figure}

\begin{figure}[t]
	\includegraphics[width=3.4in]{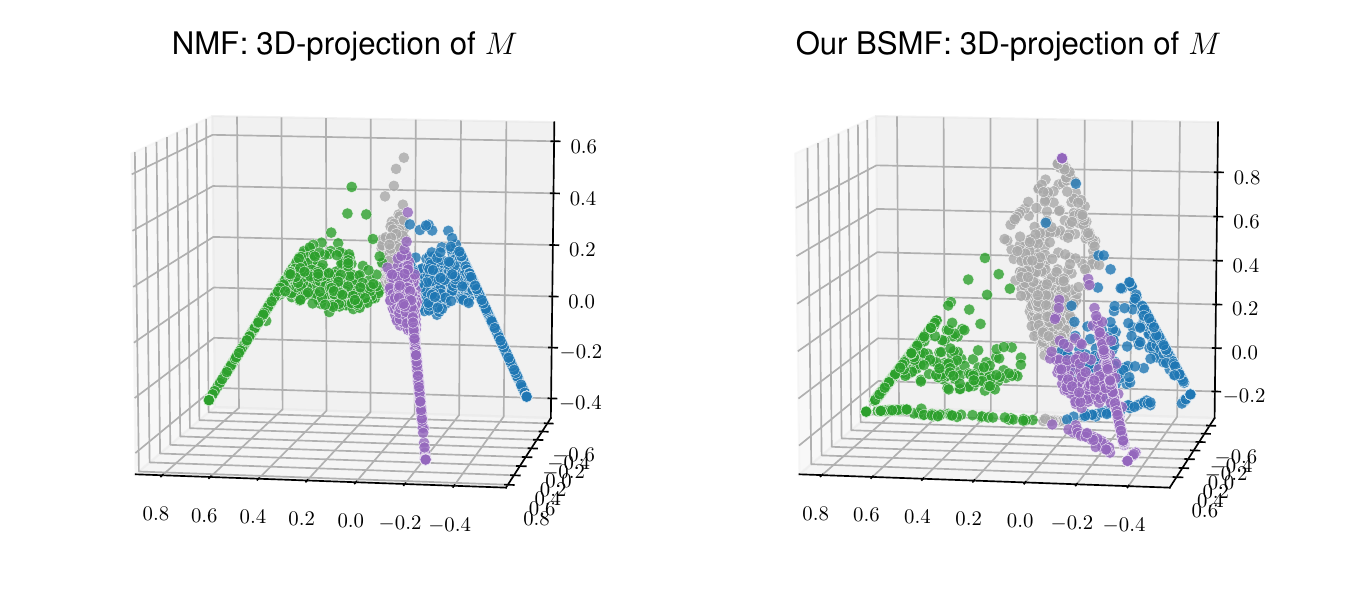}
	\vspace{-0.1in}
	\caption{Visualization of $M$ for NMF (Left) and Our BSMF (Right)}
	\label{fig:scatter}
\end{figure}
